# Supplementary material for: Deep Active Learning Using Barlow Twins
Source: arXiv:2212.14658 source file (2022-12-30)
Supplement: Supplementary file 1 [file supplament.tex]

\documentclass{article}
\usepackage[preprint]{icml2021}
% If your paper is accepted, change the options for the package
% aistats2021 as follows:
%
%\usepackage[accepted]{aistats2021}
%
% This option will print headings for the title of your paper and
% headings for the authors names, plus a copyright note at the end of
% the first column of the first page.

\usepackage{graphicx}
\usepackage{graphicx}
\usepackage[algo2e]{algorithm2e}
\usepackage{ifthen}
\usepackage{algorithm}
\usepackage{algpseudocode}
\usepackage[export]{adjustbox}
\usepackage{tabularx}

% \usepackage{array}
% \usepackage{xcolor}
% \usepackage{amsfonts}

% If you set papersize explicitly, activate the following three lines:
%\special{papersize = 8.5in, 11in}
%\setlength{\pdfpageheight}{11in}
%\setlength{\pdfpagewidth}{8.5in}

% If you use natbib package, activate the following three lines:
%\usepackage[round]{natbib}
%\renewcommand{\bibname}{References}
%\renewcommand{\bibsection}{\subsubsection*{\bibname}}

% If you use BibTeX in apalike style, activate the following line:
\bibliographystyle{apalike}

\begin{document}

% If your paper is accepted and the title of your paper is very long,
% the style will print as headings an error message. Use the following
% command to supply a shorter title of your paper so that it can be
% used as headings.
%
%\runningtitle{I use this title instead because the last one was very long}

% If your paper is accepted and the number of authors is large, the
% style will print as headings an error message. Use the following
% command to supply a shorter version of the authors names so that
% they can be used as headings (for example, use only the surnames)
%
%\runningauthor{Surname 1, Surname 2, Surname 3, ...., Surname n}

% Supplementary material: To improve readability, you must use a single-column format for the supplementary material.
\onecolumn
\icmltitle{Deep Active Learning via Open-Set Recognition - Supplementary Material}

\section{Algorithms}
\begin{algorithm}
  \SetKwData{Left}{left} \SetKwData{This}{this} \SetKwData{Up}{up}
  \SetKwFunction{Union}{Union} \SetKwFunction{FindCompress}{FindCompress}
  \SetKwInOut{Input}{input} \SetKwInOut{Output}{output} \SetKwInOut{Parameter}{}
  % $\mathcal{D}=\left\{\left(\boldsymbol{x}_{i},y_{i}\right)\right\}_{i=1}^{N}$ partioned into u
  \textbf{Input}: Unlabeled pool $\mathcal{U}^0$,labeled pool $\mathcal{L}^0$
  for $t \in\{0,1, \ldots\}$ where size of  $\mathcal{L}^0 = m_0$.\\
  \textbf{Require:} Active Learning Model, Optimizer, Sampling Strategy\\
  \textbf{Require:} initialize $b$ (budget), $\theta$ (Model parameters), Epochs\\
  \Repeat{stopping criterion (size of Labeled Pool $(\mathcal{L}^{t})$  equals 40\% of $D_{train}$)}{
    Train Active Learning Model on Labeled Pool $(\mathcal{L}^{t})$ using
    selected optimizer.\\
    Give trained model $f_\theta$ on Labeled Pool $(\mathcal{L}^{t})$, Sampling
    Strategy  (\ref{alg:samplingmethod2})  (\ref{alg:samplingmethod1})  selects the uncertain
    data points according to budget size $b$.\\
    Send the selected data points to Oracle for annotation.\\
    % Request the Oracle for target classes of the selected data points.\\
    Add the annotated data points to the Labeled Pool $(\mathcal{L}^{t})$
    }
  \caption{Active Learning}\label{alg:csm_algo}
\end{algorithm}

\begin{algorithm}[H]
  \centering
  \caption{Sampling Strategy}\label{alg:samplingmethod1}
  \footnotesize
  \begin{algorithmic}[1]
    \State \textbf{Input:} Unlabeled Pool $\mathcal{U}$, Active Learning Model ($f_\theta$), Budget b.
    \State \textbf{Output}: Set of b annotated samples $\{(x_i,y_i)\}^b$ for $i \in\{0,1, \ldots,b\}$. 
    % $\mathcal{D}_{train}=\left\{\left(\boldsymbol{x}_{i}, y_{i}\right)\right\}_{i=1}^{N}$
    \State \text {Select b samples from Unlabeled pool $\mathcal{U}$ with $min_b\{{f_{\theta}(z_{U})}\}$} 
    %  {with}$min_b\{{\theta_{TN}(z_{U})}\}$ \State \text {} $Y_{o} \leftarrow\mathcal{ORACLE}(X_{s})$ 
    % \State \text{ Add Labeled data samples intolabeled pool.} $(X_{L}, Y_{L}
    % \leftarrow (X_{L}, Y_{L}) \cup (X_{s},Y_{o})$ 
    \State \text{ \textbf{return} Annotated Samples $\{(x_i,y_i)\}^b$  }
  \end{algorithmic}
\end{algorithm}

\begin{algorithm}[H]
  \centering
  \caption{Weibull Sampling}\label{alg:samplingmethod2}
  \footnotesize
  \begin{algorithmic}[1]
    \State   \textbf{Input}: Unlabeled Pool $\mathcal{U}$, Labeled pool $\mathcal{L}$, Active Learning Model $f_\theta$, Budget b.
    \State \textbf{Output}: Set of b annotated samples $\{(x_i,y_i)\}^b$ for $i \in\{0,1, \ldots,b\}$. 
    \State \textbf{Step 1 :} 
    % samples from the approximate posterior $\boldsymbol{z}(\boldsymbol{x}^{(i)})
    % \simq_{\boldsymbol{\theta}}(\boldsymbol{z} | \boldsymbol{x}^{i})$ 
    For each data point $\boldsymbol{x}^{(i)}$ in labeled pool $\mathcal{L}$ calculate Classifier probabilities $ p_{\xi}(\boldsymbol{y} | \boldsymbol{x_i})$ 
    \State \textbf{Step 2 :} For each class $c$, let
    $\boldsymbol{S}_{c}^{(i)}$ =
    $\boldsymbol{z}(\boldsymbol{x}_{c}^{\prime(i)})$ for each correctly
    classified training example $\boldsymbol{x}_{c}^{\prime}$ 
    \State \textbf{Step 3:} \For{$c=1 \ldots C $}{\\\hspace{17mm}\textbf{Get perclass latent mean}
    $\overline{\boldsymbol{S}}_{c}=\operatorname{mean}(\boldsymbol{S}_{\underline{c}}^{(i)})$
    \\\hspace{17mm}  Weibull model  $\boldsymbol{\rho}_{c}=$ Fit Weibull
    $(||\boldsymbol{S}_{c}-\overline{\boldsymbol{S}}_{c}||, \eta)$ }

    \State For a novel data point $ \hat{x} $  in UnLabeled pool $\mathcal{U}$ calculate latent vector $ z \sim q_{\theta}(z | \hat{x})
    $  \State  Compute distances to correctly classified latent means $\overline{\boldsymbol{S}}_{c}:
    d_{c}=||{\boldsymbol{S}}_{c}-\boldsymbol{z}|| $  \\
    \For{$c=1 \ldots C $}{\\\hspace{10mm} \textbf{Weibull CDF} $
    \omega_{c}(d_{c})=1-\exp
    (-\frac{||d_{c}-\tau_{c}||}{\lambda_{c}})^{\kappa_{c}} $ }
    \State \text Select b samples from Unlabeled pool $\mathcal{U}$  { with }$max_b\{{f_{\theta}(z_{U})}\}$ 
    % \State \text{ Add Labeled data samples into labeled pool.} $(X_{L}, Y_{L} \leftarrow (X_{L}, Y_{L}) \cup (X_{s}, Y_{o})$ \State \text{
    \State \text{ \textbf{return} Annotated Samples $\{(x_i,y_i)\}^b$  }
  \end{algorithmic}
\end{algorithm}
\clearpage

\section{Datasets}

\begin{table}[hbt!]
\begin{tabular}{|c|c|c|c|c|c|c|c|c|}
\hline Dataset & #Classes & Train + Val & Test & Initially Labeled & Budget & Image Size & Batch Size & Epochs \\
\hline \hline CIFAR10  & 10 & $45000+5000$ & 10000 & 5000 & 2500 & $32 \times 32$ & 64 & 150\\
\hline CIFAR100  & 100 & $45000+5000$ & 10000 & 5000 & 2500 & $32 \times 32$ & 64 & 150\\
\hline MNIST  & 10 & $45000+5000$ & 10000 & 5000 & 2500 & $32 \times 32$ & 128 & 50\\
\hline
\end{tabular}
\caption{A summary of the datasets used in our experiments CIFAR10, CIFAR100, MNIST.}
\end{table}

\begin{table}[hbt!]
\centering
\begin{tabular}{|l|c|c|c|c|}
\hline Dataset & Learning Rate & Latent Vector Size & Model M1 & Model M2  \\
\hline \hline CIFAR10  & 0.001 &60 & VGG-16 & \shortstack{ VGG-16 (Encoder) and \\ 14-layer residual networks(decoder) } \\
\hline CIFAR100  & 0.001  & 60 & VGG-16 &\shortstack{ VGG-16 (Encoder) and \\ 14-layer residual networks(decoder) }\\
\hline MNIST  & 0.001 &60 & LeNet & - \\
\hline
\end{tabular}
\caption{A summary of the Hyperparameters used in our experiments CIFAR10, CIFAR100, MNIST.}
\end{table}

\end{document}
