# Supplementary material for: Deep Active Learning Using Barlow Twins
Source: arXiv:2212.14658 source file (2022-12-30)
Supplement: Supplementary file 2 [file supplmaentary_material.tex]

%%%%%%%% ICML 2021 EXAMPLE LATEX SUBMISSION FILE %%%%%%%%%%%%%%%%%

\documentclass{article}

% Recommended, but optional, packages for figures and better typesetting:
% Recommended, but optional, packages for figures and better typesetting:
\usepackage{microtype}
\usepackage{graphicx}
\usepackage{amsmath}
\usepackage{booktabs} % for professional tables
\usepackage{subfig}
\usepackage[algo2e]{algorithm2e}
\usepackage{amsfonts}
\usepackage{float}
\usepackage{fnpos} % \makeFNbelow by
% hyperref makes hyperlinks in the resulting PDF.
% If your build breaks (sometimes temporarily if a hyperlink spans a page)
% please comment out the following usepackage line and replace
% \usepackage{icml2021} with \usepackage[nohyperref]{icml2021} above.
\usepackage{hyperref}

% Attempt to make hyperref and algorithmic work together better:

% Use the following line for the initial blind version submitted for review:
\usepackage{icml2021}
% Use the following line for the initial blind version submitted for review:

% If accepted, instead use the following line for the camera-ready submission:
%\usepackage[accepted]{icml2021}

% The \icmltitle you define below is probably too long as a header.
% Therefore, a short form for the running title is supplied here:
\icmltitlerunning{Deep Active Learning via Open-Set Recognition Supplementary Material}

\begin{document}

\twocolumn[
\icmltitle{Deep Active Learning via Open-Set Recognition Supplementary Material}

% It is OKAY to include author information, even for blind
% submissions: the style file will automatically remove it for you
% unless you've provided the [accepted] option to the icml2021
% package.

% List of affiliations: The first argument should be a (short)
% identifier you will use later to specify author affiliations
% Academic affiliations should list Department, University, City, Region, Country
% Industry affiliations should list Company, City, Region, Country

% You can specify symbols, otherwise they are numbered in order.
% Ideally, you should not use this facility. Affiliations will be numbered
% in order of appearance and this is the preferred way.
\icmlsetsymbol{equal}{*}

\begin{icmlauthorlist}
% \icmlauthor{Aeiau Zzzz}{equal,to}
% \icmlauthor{Bauiu C.~Yyyy}{equal,to,goo}
% \icmlauthor{Cieua Vvvvv}{goo}
% \icmlauthor{Iaesut Saoeu}{ed}
% \icmlauthor{Fiuea Rrrr}{to}
% \icmlauthor{Tateu H.~Yasehe}{ed,to,goo}
% \icmlauthor{Aaoeu Iasoh}{goo}
% \icmlauthor{Buiui Eueu}{ed}
% \icmlauthor{Aeuia Zzzz}{ed}
% \icmlauthor{Bieea C.~Yyyy}{to,goo}
% \icmlauthor{Teoau Xxxx}{ed}
% \icmlauthor{Eee Pppp}{ed}
\end{icmlauthorlist}

\icmlaffiliation{to}{Department of Computer Science, Georgia State University, Georgia, US}
% \icmlaffiliation{goo}{Googol ShallowMind, New London, Michigan, USA}
% \icmlaffiliation{ed}{School of Computation, University of Edenborrow, Edenborrow, United Kingdom}

\icmlcorrespondingauthor{Jaya Krishna Mandivarapu}{jmandivarapu1@student.gsu.edu}
\icmlcorrespondingauthor{Blake Camp}{bcamp2@student.gsu.edu}
\icmlcorrespondingauthor{Rolando Estrada}{restrada1@gsu.edu}
% You may provide any keywords that you
% find helpful for describing your paper; these are used to populate
% the "keywords" metadata in the PDF but will not be shown in the document
\icmlkeywords{Machine Learning, ICML}

\vskip 0.3in
]

% this must go after the closing bracket ] following \twocolumn[ ...

% This command actually creates the footnote in the first column
% listing the affiliations and the copyright notice.
% The command takes one argument, which is text to display at the start of the footnote.
% The \icmlEqualContribution command is standard text for equal contribution.
% Remove it (just {}) if you do not need this facility.

%\printAffiliationsAndNotice{}  % leave blank if no need to mention equal contribution
\printAffiliationsAndNotice{\icmlEqualContribution} % otherwise use the standard text.

\begin{abstract}

 In many applications, data is easy to acquire but expensive and time-consuming to label---prominent examples include medical imaging and NLP. This disparity
  has only grown in recent years as our ability to collect data improves. Under
  these constraints, it makes sense to select only the most informative
  instances from the unlabeled pool and request an oracle (e.g., a human expert)
  to provide labels for those samples. The goal of active learning is to infer
  the informativeness of unlabeled samples so as to minimize the number of
  requests to the oracle. Here, we formulate active learning as an open-set
  recognition problem. In this paradigm, only some of the inputs belong
  to known classes; the classifier must identify the rest as \textit{unknown.}
  More specifically, we leverage variational neural networks (VNNs), which
  produce high-confidence (i.e., low-entropy) predictions only for inputs that
  closely resemble the training data. We use the inverse of this confidence
  measure to select the samples that the oracle should label. Intuitively,
  unlabeled samples that the VNN is uncertain about are more informative for
  future training. We carried out an extensive evaluation of our novel,
  probabilistic formulation of active learning, achieving state-of-the-art
  results on MNIST, CIFAR-10, and CIFAR-100. Additionally, unlike current active learning
  methods, our algorithm can learn tasks without the need for task labels. As our experiments show, when the unlabeled pool
  consists of a mixture of samples from multiple datasets, our approach can
  automatically distinguish between samples from seen vs. unseen tasks.
\end{abstract}

\section{Introduction}
Supervised deep learning has achieved remarkable results across a variety of
domains by leveraging large, labeled datasets \cite{LeCun2015}. However, our
ability to collect data far outstrips our ability to label it, and this
difference only continues to grow. This problem is especially stark in
domains where acquiring the ground truth requires a highly trained specialist, e.g., medical imaging. Even in cases where labeled data is sufficient, there may be reasons to limit the amount of data used to train a model, e.g., time, financial constraints, or to minimize the model's carbon footprint.

Fortunately, the relationship between a model's performance and the amount of
training data is not linear. There often exists a small subset of highly
\textit{informative} samples that can provide most of the information needed to
learn to solve a task. In this case, we can achieve nearly the same performance
by labeling (and training on) only those informative samples, rather than the
entire dataset. The challenge, of course, is that the true usefulness of a
sample can only be established \textit{a posteriori}, after we have used it to
train our model.

\begin{figure*}[t]
  \centering
    \includegraphics[width=0.8\textwidth]{images/Active Learning}
  \caption{\textbf{Framework overview:} Our proposed active learning system uses open-set recognition to identify which samples from the unlabeled pool to label. Our classifier is a variational neural network (VNN) \cite{Mundt2019OpenSR}, which simultaneously reconstructs an input using a probabilistic autoencoder (AE) and classifies it by feeding the AE's latent vector $z$ to a linear classifier. We use the VNN's loss function to determine which samples to select from the unlabeled pool (Sample Selection). As in \cite{Mundt2019OpenSR}, we tested two VNN variants: M1 is trained using only the loss on the latent vector $q_\Phi(z|x)$ and the classifier $p(y|z)$, while M2 also includes the loss on the reconstructed input $p_\Phi(x|z)$. Figure based on similar diagrams in \cite{Mundt_UnifiedOSR} and \cite{sinha2019variational}.}
  \label{fig:overview}
\end{figure*}

% Our proposed system has two models $M_i$ which we call M1 and M2 from now \textbf{a)} Encoder followed by a linear classifier (M1) \textbf{b} Encoder with Decoder Architecture (M2). Selected Model will be trained on initial labeled pool $\mathcal{L}$ samples. Once the initial training stage finishes on labeled pool $\mathcal{L}$, our selector will be given unlabeled pool $\mathcal{U}$ and trained Model. Our sampling module $\mathcal{S}$ will return most informative samples that needs to be sent to oracle for annotation according to the budget size available. After the annotation those annotated images will be removed from unlabeled pool $\mathcal{U}$, added to labeled pool $\mathcal{L}$.
   
% As such, we need a way to predict which unlabeled samples are worth labeling.

The growing field of \textit{active learning} (AL) is concerned with
automatically predicting which samples from an unlabeled dataset are most worth
labeling.\footnote{As noted in \cite{sinha2019variational}, active learning can
also refer to approaches that generate or synthesize novel samples. In this
paper, however, we will only be concerned with sampling-based active learning.}
In the standard AL framework, a selector identifies an initial set of promising
samples; these are then labeled by an oracle (e.g., a human expert) and used to
train a task network \cite{gal2017deep}. The selector then progressively
requests labels for additional batches of samples, up to either a percentage
threshold (e.g., 40\% of the total data) or until a performance target is met.
In short, an active learning system seeks to construct the smallest possible
training set which will produce the highest possible performance on the
underlying task/s.

In this paper, we formulate active learning as an \textit{open-set recognition
(OSR) problem}, a generalization of the standard classification paradigm. In OSR,
only some of the inputs are from one of the known classes; the classifier must
label the remaining inputs as \textit{out-of-distribution (OOD)} or
\textit{unknown}. Intuitively, our hypothesis is that the samples most worth
labeling are those that are most different from the currently labeled pool.
Training on these samples will allow the network to learn features that are
underrepresented in the existing training data. In short, our AL selection
mechanism consists of picking unlabeled samples that are OOD relative to the
labeled pool.

% OSR requires novel classification methods because traditional approaches have
% no mechanism to distinguish known from unknown classes. In fact, deep neural
% networks have been shown to yield high-confidence outputs for nonsense inputs
% (e.g., classifying random dots as a penguin with 99.9\% confidence)
% [CITATION].

Figure~\ref{fig:overview} illustrates our proposed approach. In more detail, our
classifier is a variational neural network (VNN) \cite{Mundt2019OpenSR}, which
produces high-confidence (i.e., low-entropy) outputs only for inputs that are
highly similar to the training set. We use the inverse of this confidence
measure to select which unlabeled samples to query next. In other words, our
selector requests labels for the samples that the classifier is \textit{least
confident} about because this implies that the existing training set does not
contain items that are similar to them. As we detail in
Sec.~\ref{sec:experiments}, our OSR-based approach achieved state-of-the-art
results in a number of datasets and AL variations, far surpassing existing
methods.

The rest of this paper is organized as follows. In Sec.~\ref{sec:relatedWork},
we provide a brief overview of current active learning and open-set recognition
methods. In Sec.~\ref{sec:methodology}, we present our proposed approach, then
detail our experiments in Sec.~\ref{sec:experiments}. Finally, we discuss
avenues for future work in Sec.~\ref{sec:conclusions}.

% As noted in \cite{sinha2019variational}, recent approaches to the problem of active learning can be broadly categorized as query-acquiring or query-synthesizing. The distinction lies in whether informative samples are immediately accessible in the unlabeled pool and must therefore merely be selected for labeling (query-acquiring); or, must instead be synthesized using a generative model (query-synthesizing) \cite{AL_usingSampleSelectionConditionalGenerativeAdversarialNetwork, AdversarialSamplingForActiveLearning, DBLP:journals/corr/ZhuB17}. Since our work adheres to the query-acquisition paradigm, we will focus mainly on similar sampling approaches. 

% The learned model is, in essence, an intelligent sampling function, or strategy, the aim of which is to outperform random sampling of the unlabeled distribution. 

\section{Related Work}
\label{sec:relatedWork}
\subsection{Sampling-based active learning}
It has been shown that training samples do not contain equal amounts of useful information \cite{activeLearningLitSurvey}. Thus, the goal of sampling-based active learning is to learn an \textbf{\textit{acquisition function}} that chooses the best data points for which a label should be requested from a large, unlabeled pool of data \cite{gal2017deep}. There have been numerous efforts to learn an optimal sampling strategy, and they can be broadly grouped into three major categories \cite{sinha2019variational}.  Uncertainty-based techniques aim to select samples from the unlabeled distribution about which the current classifier is highly uncertain.  Representations-based models aim to maximize quantifiable \textit{diversity} in training batches \cite{sener2017active}.  Finally, hybrid approaches attempt to combine quantifiable uncertainty and diversity in order to select training samples \cite{adaptiveActiveLearningForImageClassification}. VAAL \cite{sinha2019variational} proposed an adversarial learning based method in which a discriminator is trained along with the task network to discriminate whether an example belongs to the labeled or unlabeled set. In \cite{sener2017active}, the authors considered active learning as a set-cover problem, one in which a task network is trained using a core-set loss, which is the difference between a task-network's classification error over the labeled set vs. the core-set. DBAL \cite{gal2017deep} approached the active learning problem using Bayesian convolutional neural networks, wherein confidence is measured using variation ratios. In MC-Dropout \cite{gal2016dropout}, the authors proposed to model the uncertainty present in deep networks by interpreting dropout as a type of Bayesian inference in deep Gaussian processes.

% thereby attempting to maximize the learning efficiency of the system.  

% As such, various sampling strategies have been proposed which can typically be grouped into three broad categories \cite{sinha2019variational}. They include uncertainty-based techniques, representation-based models \cite{sener2017active}, and hybrid approaches \cite{DBLP:conf/icml/NguyenS04}.

% Assuming
% access to a pool of unlabeled OOD data, a strategy must be devised which selects
% only the most useful or informative samples from that distribution. 

% In other words, some
% training distributions result in better task performance than others.  Thus, the
% aim of an active learning system is to minimize the amount of training data
% required to achieve the highest possible performance on an underlying task, e.g.
% image classification. This is a form of learning efficiency, which we wish to
% improve, or maximize.  

% \textbf{Open-set recognition}
% \textcolor{blue}{"In \cite{activeLabelingForDL}, an AL model was developed for
% DL using three metrics for data sampling: least confidence, margin sampling,
% and entropy" \cite{shi2020evidenceaware}}.  \textcolor{blue}{"Another approach
% advances the AL development by introducing a cost-effective strategy to
% automatically select and annotate the high-confidence samples, which improves
% the traditional samples selection strategies"
% \cite{DBLP:journals/corr/WangZLZL17}}.

\subsection{Open-set recognition}
Open-Set Recognition (OSR) refers to the ability of a system to distinguish between types of data it has already seen (the training distribution) from types to which it has not yet been exposed (out-of-distribution (OOD) data). Standard deep neural networks are not suitable for OSR because they often yield high confidence values for inputs which are significantly different from the training classes. As noted by \cite{PMID:32191881}, existing OSR methods can be subdivided into discriminative-based and generative-based approaches. Discriminative methods modify traditional ML and deep neural networks to tackle the OSR problem. For example, \cite{scheirer2012toward} used traditional SVMs with an additional open space risk term, while \cite{zhang2016sparse} extended sparse classifiers to OSR by modeling the error distribution using Extreme Value Theory (EVT) \cite{vignotto2018extreme}. Some other discriminative methods use nearest neighbors \cite{junior2017nearest}, probability models  \cite{jain2014multi,scherreik2016open,scheirer2014probability}, or outlier detection \cite{bendale2015towards}. 

Generative methods primarily use generative adversarial networks (GANs) \cite{2017arXiv170100160G} for OSR. For example, \cite{neal2018open} proposed G-OpenMax by adopting an encoder-decoder GAN architecture for generating samples which are highly similar to training samples yet do not belong to any of the training classes. Following a similar approach, \cite{yang2019open} investigated the open-set human activity recognition problem based on micro-Doppler signatures by using a GAN to generate samples which were highly similar to the target class and forming a negative set out of it. Not all generative approaches use GANs, though. For example, \cite{geng2018collective} proposed a collective, decision-based OSR model by slightly modifying the hierarchical Dirichlet process.

\section{Methodology} \label{sec:methodology}
As noted above, our active learning approach iteratively selects samples from an
unlabeled pool based on the confidence level of its OSR classifier. Below, we
first formalize the active learning paradigm we are tackling, then detail our
proposed system. In particular, we provide an overview of VNNs and explain how
we use their outputs to select new samples to label.

\subsection{Formal problem definition} \label{sec:overview} 
Formally, an active learning problem is denoted as $P = (C, D_{train}, D_{eval})$, where $C$ indicates the number of classes, $D_{train}$ is the training set, and $D_{eval}$ is the evaluation set, s.t.
$D_{train} \cap D_{eval} = \emptyset $.

Let $\mathcal{D}_{train}=\left\{\left(\boldsymbol{x}_{i}, y_{i}\right)\right\}_{i=1}^{N}
$ be a dataset consisting of $N$ i.i.d. data points where only
$m$ of them are labeled ($m$\(<\!\!<\)$N$). Each sample \(
\boldsymbol{x}_{i} \in \mathbb{R}^{d} \) is a $d$-dimensional feature vector, and
\( y_{i} \in\{1,2, \ldots, C\} \) represents the target label. 
% The $m$ labeled samples are
% uniformly sampled subset from the $N$ samples.
At the start, $\mathcal{D}_{train}$ is partitioned into two disjoint subsets: a labeled set
$\mathcal{L}$ which consists of the $m$ labeled data points, and 
an unlabeled set $\mathcal{U}$ which consists of the remaining $N-m$ data points with unknown
target labels. We will update both $\mathcal{L}$ and $\mathcal{U}$ after each iteration of our algorithm. We denote the state of a subset at a given timestep as $\mathcal{L}^t$
and $\mathcal{U}^t$, respectively, for $t \in\{0,1, \ldots\}$. 

% Active learning begins with a set of $m_0$ labeled samples, which we denote $\mathcal{L}^0$. 

In active learning, we first train a classifier $f$, with parameters $\theta$, on $\mathcal{L}^0$. Afterwards we select $b$ data points from $\mathcal{U}^0$ using our OSR criterion (see Sec.~\ref{sec:ALSystem}). These $b$ data points are then sent to the oracle for annotation. The annotated samples are removed from the unlabeled pool and added to the labeled pool, along with their newly acquired target labels. The updated labeled and unlabeled data pools become $\mathcal{L}^1$, of size $m+b$, and $\mathcal{U}^1$, respectively. Thus, the labeled pool grows in size as training progresses. We continue
this process until the size of the labeled pool reaches a predefined limit (40\% of $D_{train}$ in our experiments).

% , whereby $\mathcal{L}^0 \subset \mathcal{L}^1 \subset .... \mathcal{L}^t$, which have respective sizes  $m_0$\(<\!\) $m_1$ \(<\!\) $m_2$....\(<\!\) $m_t$ 

% Finally, we train a classifier $f$ with parameters $\theta$ on the
% labeled pool $\mathcal{L}^1$.
% In each subsequent iteration, we use our OSR
% criterion (see Sec.~\ref{sec:ALSystem}) to select $b$ additional data samples
% from $\mathcal{U}$. We query the labels of these new samples, add them to
% $\mathcal{L}$, and train our classifier on all the labeled data. 

Importantly, unlike other formulations of AL, we allow for the unlabeled pool $\mathcal{U}$ to contain training data from \textit{multiple datasets}. As we show in our experiments, our OSR-based AL method can automatically ignore samples that do not belong to the target classes.

% In addition, we assume no task IDs. Our OSR selection criterion allows our system to learn multiple tasks without specifying the
% current task.

% This has clear limitations when the i.i.d assumption is not satisfied or when the task boundaries are not available.
\begin{algorithm}
  \SetKwData{Left}{left} \SetKwData{This}{this} \SetKwData{Up}{up}
  \SetKwFunction{Union}{Union} \SetKwFunction{FindCompress}{FindCompress}
  \SetKwInOut{Input}{input} \SetKwInOut{Output}{output} \SetKwInOut{Parameter}{}
  % $\mathcal{D}=\left\{\left(\boldsymbol{x}_{i},y_{i}\right)\right\}_{i=1}^{N}$ partioned into u
  \textbf{Input}: Unlabeled pool $\mathcal{U}^0$, labeled pool $\mathcal{L}^0$
  for $t \in\{0,1, \ldots\}$ where size of  $\mathcal{L}^0 = m_0$.\\
  \textbf{Require:} Active Learning Model, Optimizer, Sampling Strategy\\
  \textbf{Require:} initialize $b$ (budget), $\theta$ (Model parameters), Epochs\\
  \Repeat{stopping criterion (size of Labeled Pool $(\mathcal{L}^{t})$  equals 40\% of $D_{train}$)}{
    Train Active Learning Model on Labeled Pool $(\mathcal{L}^{t})$ using
    selected optimizer.\\
    Give trained model $f_\theta$ on Labeled Pool $(\mathcal{L}^{t})$, Sampling
    Strategy  (\ref{sec:uncertaintySampling} or  \ref{sec:WiebullSampling})  selects the uncertain
    data points according to budget size $b$.\\
    Send the selected data points to Oracle for annotation.\\
    % Request the Oracle for target classes of the selected data points.\\
    Add the annotated data points to the Labeled Pool $(\mathcal{L}^{t})$
    }
  \caption{Active Learning}\label{alg:csm_algo}
\end{algorithm}
\subsection{Active learning system}
\label{sec:ALSystem}
Algorithm~\ref{alg:csm_algo} summarizes our AL approach, which has two main components: a variational
neural network (VNN) \cite{Mundt2019OpenSR} that serves as our classifier and an OSR selection mechanism based on the loss function of the VNN. We discuss each component below.

\subsubsection{Variational Neural Networks (VNNs)}
\label{sec:VNNs}
Variational neural networks (VNNs) \cite{Mundt2019OpenSR} are a supervised
variant of $\beta$-variational autoencoders ($\beta$-VAE)
\cite{higgins2017beta}. The latter is itself a variant of VAEs
\cite{tutorial_VAE} but with a regularized cost function. That is, the
cost function for a $\beta$-VAE consists of two terms: the reconstruction error,
as with a regular VAE, and an \textit{entanglement} penalty on the latent
vector. This penalty forces the dimensions of the latent space to be as
uncorrelated as possible, making them easier to interpret.

% Intuitively, That is, $\beta$-VAE are used for unsupervised learning, without
% any target labels. VNNs, on the other hand, 

% \begin{align} L(x) = L_{\text{rec}}(x,\hat{x}) + \beta L_{\text{ent}}(z).
% \end{align} Here, $x$ and $\hat{x}$ are the input and reconstructed output,
% resp., while $z$ is the latent vector.

A VNN combines the encoder-decoder architecture of a $\beta$-VAE with a
probabilistic linear classifier (see Fig.~\ref{fig:overview} for a visual
representation). As such, its loss function includes a classification error,
i.e., a supervised signal, in addition to the reconstruction and entanglement
terms:
\begin{equation}
\begin{split}
  \label{eqn:M2Loss}
  L(\theta, \phi, \xi) = \mathbb{E}_{q_{\theta}(\boldsymbol{z} | \boldsymbol{x})} &\left[{\log p_{\phi}(\boldsymbol{x} | \boldsymbol{z})} + {\log p_{\boldsymbol{\xi}}(\boldsymbol{y} | \boldsymbol{z})} \right] \\ 
  & - \beta \,\text{KL}\left(q_{\theta}(\boldsymbol{z} | \boldsymbol{x}) \| p(\boldsymbol{z})\right)
\end{split}    
\end{equation}
As detailed in \cite{Mundt2019OpenSR}, $\theta$, $\phi$, and $\xi$ are the
parameters of the encoder, decoder, and classifier, resp., while
$p_{\phi}(\boldsymbol{x} | \boldsymbol{z})$ and
$p_{\boldsymbol{\xi}}(\boldsymbol{y} | \boldsymbol{z})$ are the reconstruction
and classification terms. The last term is the entanglement penalty, which is
given by the Kullback-Leibler divergence between the latent vector distribution
and an isotropic Gaussian distribution.

As in \cite{Mundt2019OpenSR}, we evaluated both the full framework discussed above (dubbed $M_2$
in our experiments), which uses the loss function in Eq.~\ref{eqn:M2Loss}, and a
simplified version ($M_1$) without the reconstruction error:
\begin{equation}
  \label{eqn:M1Loss}
  L(\theta, \xi)= \mathbb{E}_{q_{\theta}(\boldsymbol{z} | \boldsymbol{x})} \left[{\log p_{\boldsymbol{\xi}}(\boldsymbol{y} | \boldsymbol{z})} \right] -\beta \,\text{KL}\left(q_{\theta}(\boldsymbol{z} | \boldsymbol{x}) \| p(\boldsymbol{z})\right)
\end{equation}
As our experiments show, both versions 
outperform the state of the art, but
$M_2$ achieves better results overall.

\subsubsection{Sample Selection}
\label{sec:Sampling}
We wish to leverage the class disentanglement penalty defined in  Eq.~\ref{eqn:M2Loss}. Specifically, our aim is to select $b$ data points from the unlabeled pool $\mathcal{U}$ that the VNN is highly uncertain about. Following \cite{Mundt_UnifiedOSR}, in our experiments we investigated two sampling algorithms for OSR: \textit{uncertainty sampling} and \textit{Weibull distribution sampling}. The former is simpler, but the latter allows one to better reject outliers. We briefly describe each sampling strategy below.

% \noindent \textbf{Uncertainty Sampling} :

\subsection{Uncertainty sampling}
\label{sec:uncertaintySampling}
Here, we select a data point $\boldsymbol{x}_i$ based directly on how uncertain the VNN is about it. Specifically, we rank all unlabeled samples by the value of the most likely class label and select the $b$ samples with the lowest maximum values. Since the sum of class likelihoods is normalized, the value of the maximum class probability will approach one for highly certain samples and approach $\frac{1}{|C|}$, where $|C|$ is the number of classes, for highly uncertain samples. In other words, the class likelihoods of uncertain samples have higher entropy than those for which the VNN is certain about.

% Model uncertainty can be measured in several ways. Our approach captures our model's epistemic or prediction uncertainty for any given input $\boldsymbol{x}_\textbf{i}$ (see Algorithm~1 in the Supplementary Materials for more details). We use the prediction probability produced by the trained classifier for all the data points present in the unlabeled pool $\mathcal{U}$. The \textbf{$b$} number of informative data points are selected according to the model uncertainty which captures most of the epistemic uncertainty. The selected informative data points are 
% the entropy associated with the model’s predictions as a score to collect 
% \textbf{$b$} number of informative samples are selected by computing utility of
% the unlabeled instances in  $\mathcal{U}$ where the utility is model uncertainty.

% sent to the oracle to obtain its target label $y^\ast$. Note that the closer the probability is to
% zero, the more likely it is that the model is very uncertain about that sample.

% \noindent \textbf{Wiebull Distribution Sampling :} 

\subsection{Wiebull distribution sampling}
\label{sec:WiebullSampling}
As our experiments show, uncertainty sampling is suitable for active learning problems in which all unlabeled samples belong to known classes. However, for the case where the unlabeled pool also contains samples from unknown classes, we need a more robust way to exclude outliers. For this latter case, we employed the sampling procedure defined in \cite{Mundt_UnifiedOSR}, which leverages a Wiebull distribution to estimate the model's uncertainty w.r.t a specific sample. 

For completeness, here we will briefly outline the methodology proposed in \cite{Mundt_UnifiedOSR}. Intuitively, it can be shown that it is useful to quantify the probability that a given data sample is an outlier, herein defined as a sample which is not sufficiently similar to those which have already been correctly classified.  \cite{Mundt_UnifiedOSR} show that this can be accomplished as follows. First, for each class, we compute the mean of the latent vectors of all samples that have been correctly predicted by the model. Second, we compute the distances from each class mean for all latent vectors, which \cite{Mundt_UnifiedOSR} showed can be modeled with a Wiebull distribution. As such, a sample's likelihood under this distribution constitutes the minimum probability that the sample does \textbf{\textit{not}} belong to any previously known class. In other words, the lower this value, the more likely that the sample is an outlier.

\section{Experimental Results}
\label{sec:experiments}
We performed experiments on three image classification datasets---MNIST, CIFAR-10, and CIFAR-100---following the methodology defined in Section \ref{sec:methodology}. Below, we first present our implementation details, then discuss our results.

\begin{figure}[h]%
    \centering
    \subfloat[\centering ]{{\includegraphics[width=6.5cm]{images/final_MNIST_100.png} }}%
    \qquad
    \subfloat[\centering ]{{\includegraphics[width=6.5cm]{images/final_MNIST.png} }}%
     \caption{Performance on MNIST classification tasks using different query sizes for model $M_1$. (a) Query batch size
of 100; (b) Query batch size of 1000 compared
  to Core-set \cite{sener2017active}, DBAL \cite{gal2017deep}, Random Sampling and Uncertainty Sampling. M1
  indicates our model with Encoder and Classifier. Best visible in color. Prior results adapted from \cite{sinha2019variational}.} %
    \label{fig:MNIST}%
    
\end{figure}

\begin{figure*}[]
  \centering
  \includegraphics[width=15cm]{images/CF10-100.png}
  \caption{ Performance on classification tasks for CIFAR-10 (left) and CIFAR-100 (right)
  compared to VAAL \cite{sinha2019variational}, Core-set \cite{sener2017active},
  Ensembles w. VarR \cite{powerOfEnsemblesForActiveLearning}, MC-Dropout
  \cite{gal2016dropout}, DBAL \cite{gal2017deep}, and Random Sampling. M1
  indicates our model \eqref{eqn:M1Loss} and M2 indicates our model
  \eqref{eqn:M2Loss}. All the legend names are in descending order of final accuracies. Best visible in color. Prior results adapted from \cite{sinha2019variational}.}
  \label{fig:CF10CF100}
\end{figure*}

% \subsection{Bias, Budgets, and Noise}
% In the following sections, we replicate and extend the experiments of the same name put forth in \cite{sinha2019variational} in order to compare our approach with other state-of-the-art techniques. 

\subsection{Implementation Details} \label{Implementation}

\textbf{Budget:} For CIFAR-10  and  CIFAR-100, we used a max budget of 40\%, and stage budgets $b$ of 10\%, 15\%, 20\%, 25\%, 30\%, 35\%, and 40\%.  For MNIST, we used stage budgets of 100 and 1000 images. 

% We do not have results for 250 MNIST.

\textbf{Runs:} For all three datasets, we measured performance by computing the average accuracy across 5 independent runs.

\textbf{State of the art comparison}: We compared our method against several recent AL approaches including Variational Adversarial Active Learning (VAAL) \cite{sinha2019variational}, Core-Set  \cite{sener2017active}, Monte-Carlo Dropout \cite{gal2016dropout}, Ensembles using Variation Ratios (Ensembles w. VarR ) \cite{freeman1965elementary} \cite{powerOfEnsemblesForActiveLearning}, and Deep Bayesian AL (DBAL) \cite{gal2017deep}. As a baseline, we also included uniform random sampling (Random) since it remains a competitive strategy in the field of active learning.

% which employs a  sampling strategy that leverages a max entropy metric, and is used to quantify the model's uncertainty. 

\textbf{Architectures:} For experiments on CIFAR-10 and CIFAR-100 we used a VGG16 network \cite{simonyan2014very} as the encoder for both models, $M_1$ and $M_2$, and a decoder based on 14-layer residual networks \cite{higgins2017beta, zagoruyko2016wide}.  We used latent vectors of size 60. As noted in Sec.~\ref{sec:methodology}, the classifier consists of a single linear layer. For MNIST, we used a LeNET network \cite{LeNET} as our encoder and a latent vector of size 60. 

\textbf{Optimization:} We optimized all models using a mini-batch size of 128, a learning rate of 0.001, and a weight decay of $10^{-5}$. We tested two different optimizer, SGD and ADAM \cite{kingma2014adam}, for both $M_1$ and $M_2$, for a total of four combinations:
\begin{itemize}
    \item $M_1^{sgd}$ - Model $M_1$ as shown in  Eq.~\ref{eqn:M1Loss} with SGD optimizer.
    \item $M_1^{adam}$ - Model $M_1$  as shown in  Eq.~\ref{eqn:M1Loss} with Adam optimizer.
    \item $M_2^{sgd}$ - Model $M_2$ as shown in  Eq.\ref{eqn:M2Loss}, with SGD optimizer.
    \item $M_2^{adam}$ - Model $M_2$ as shown in  Eq.\ref{eqn:M2Loss} with Adam optimizer.
\end{itemize}

% \textcolor{black}{For the EVT based outlier rejection, we fit Weibull models with a tail-size set to 5 \%  of training data points per class present in labeled pool $\mathcal{L}$, and the distance metric used is cosine.}

\textbf{Oracle queries:} We defined a learning stage (i.e., a period of training between queries to the oracle) as lasting 150 epochs on CIFAR-10 and CIFAR-100 and 10 epochs on MNIST. At the completion of a stage, we requested labels for $b$ images from the unlabeled pool. These were added to the labeled pool and used in the subsequent learning stages.

% For all experiments, the initial labeled pool size  was set to be 10 \%  of the complete training set, $\mathcal{D}_{train}$. 

% The budget size $b$ at each stage was set to 5 \%  of the
% $\mathcal{D}_{train}$  training set, which is equivalent to 2500, 2500 for CIFAR 10, and CIFAR 100. 

% $M_1^{sgd}$ \hspace{3mm}   - Model M1 as shown in  Eq.\ref{eqn:M1Loss} with optimizer as SGD. \\
% $M_1^{adam}$ \hspace{0mm}  - Model M1  as shown in  Eq.\ref{eqn:M1Loss} with optimizer as ADAM. \\
% $M_2^{sgd}$ \hspace{3mm}    - Model M2 as shown in  Eq.\ref{eqn:M2Loss}, with optimizer as SGD \\
% $M_2^{adam}$  \hspace{0mm}  - Model M2  as shown in  Eq.\ref{eqn:M2Loss} with optimizer as ADAM.

% \begin{figure*}
%   \centering
%   \includegraphics[scale=0.15]{images/budgets-poolbias.png}
%   \caption{ RobustnessS of our approach on classification task CIFAR100 to (a)
%   budget size (left), (b) biased initial labeled pool (right), with  compared to
%   VAAL \cite{sinha2019variational}, Core-set \cite{sener2017active} , Ensembles
%   w. VarR \cite{powerOfEnsemblesForActiveLearning}, MC-Dropout
%   \cite{gal2016dropout}, DBAL \cite{gal2017deep}, and Random Sampling. M1
%   indicates our model \eqref{eqn:M1Loss} and M2 indicates our model
%   \eqref{eqn:M2Loss}. Best visible in color. Data and code required to reproduce
%   are provided in our supplementary material.}
%   \label{fig:mixeddifferentBudgets}
% \end{figure*}

\begin{figure*}%
    \centering
    \subfloat[\centering ]{{\includegraphics[width=8cm]{images/BIASED.png} }}%
    \qquad
    \subfloat[\centering ]{{\includegraphics[width=8cm,height=7.8cm]{images/VARIOUS_BUDGETS.png} }}%
     \caption{ Robustness of our approach on CIFAR-100 given (a) biased initial labeled pool or (b)
  different budget sizes compared to
  VAAL \cite{sinha2019variational}, Core-set \cite{sener2017active} , Ensembles
  w. VarR \cite{powerOfEnsemblesForActiveLearning}, MC-Dropout
  \cite{gal2016dropout}, DBAL \cite{gal2017deep}, and Random Sampling. M1
  indicates our model \eqref{eqn:M1Loss} and M2 indicates our model
  \eqref{eqn:M2Loss}. Best visible in color. Prior results adapted from \cite{sinha2019variational}.}%
  \label{fig:mixeddifferentBudgets}%
    
\end{figure*}

% %  Data and code required to reproduce
%   are provided in our supplementary material. \textcolor{red}{we need to mention about the data taken from the VAAL official code repo. Should we mention that in the footnote itself? https://github.com/sinhasam/vaal}

\subsection{Image classification results}

% using an initial labeled pool $\mathcal{L}$ size of 100 with different budget sizes of 100, 1000 (further experimental details can be found in Appendix ). 

% For model $M_1^{sgd}$ we report performance  w.r.t to other methods such as Core-set \cite{sener2017active}, DBAL \cite{gal2017deep}, Random Sampling  and Uncertainty Sampling. 

\textbf{MNIST:} Our results were comparable with the state of the art on MNIST. However, as Figs.~\ref{fig:MNIST}(a) and  Fig.~\ref{fig:MNIST}(b) show, random sampling is already a highly successful strategy on MNIST, leaving little room for improvement on this dataset. In particular, as illustrated in Fig.~\ref{fig:MNIST}(b), all methods obtained statistically similar results as the batch size increased. However, as shown in Fig.~\ref{fig:MNIST}(a) methods such as DBAL or Coreset have lower accuracies at the initial stages when using smaller batch sizes.

\noindent \textbf{CIFAR-10 \& CIFAR-100:}  As Fig.~\ref{fig:CF10CF100} clearly shows, we achieved state-of-the-art performance by a considerable margin on both CIFAR-10 (left) and CIFAR-100 (right).

On CIFAR-10, models [$M_1^{sgd},M_1^{adam},M_2^{sgd},M_2^{adam}$] achieved mean accuracies of [84.4\%, 89.24\%, 89.97\%, 91.4\%], respectively. To put this in perspective, the original accuracy for this VNN using the entire CIFAR-10 dataset was 92.63\%. VAAL came in second, with an accuracy of only 80.71\% , followed by Core-Set with an accuracy of 80.37\%, and then Ensemble w VarR at 79.465\%.  Random sampling, DBAL and MC-Dropout all trailed significantly behind other methods. Finally, we found that our models trained with ADAM, on average, outperform those trained with SGD.

On CIFAR-100, models [$M_1^{sgd},M_1^{adam},M_2^{sgd},M_2^{adam}$]  achieved mean accuracies of [54.47\%, 60.68\%, 61.25\%, 61.93\%], resp. The original accuracy with the entire CIFAR-100 dataset was 63.14\%. VAAL once again came in second, with an accuracy of 54.47 \%, followed by Core-Set, and Ensemble w VarR. 

% The total accuracy of 92.63\% could be achieved when training on the entire dataset for CIFAR-10 and 63.14\% on CIFAR-100.

% We set a max budget of 40\% of the complete training set. 

% We trained for 6 stages. 

% As a baseline, we first established that an accuracy of 92.63\% could be achieved when training on the entire dataset, denoted as \textit{Top-1 accuracy} in Figure \ref{fig:CF10CF100} (a) (left). 

% \noindent\textbf{CIFAR100:} While our models
% [$M_1^{sgd},M_1^{adam},M_2^{sgd},M_2^{adam}$]  achieves a mean accuracy of
% [54.47\%, 60.68\%, 61.25\%, 61.93\%].  As shown in
% Fig.\ref{fig:CF10CF100} (right)  other methods which performs closest to our
% model's is VAAL with accuracy of 54.47 \%, core-set, Ensemble w VarR  with
% accuracy of  and with accuracy of 46.78\%. Moreover as shown in the figure
% Fig.\ref{fig:CF10CF100} (b)(right) the proposed  methods
% [$M_1^{adam},M_2^{sgd},M_2^{adam}$]  can achieve the top performance of VAAL
% using 20\% of the annotated training data itself and $M_1^{sgd}$ by using 30\%
% of the annotated training data. The proposed models consistently outperform the existing
% baselines.

\subsection{Additional experiments}
In addition to our classification experiments, we replicated and extended the experiments of the same name put forth in \cite{sinha2019variational} in order to investigate the robustness of our approach. Unless otherwise stated, we used CIFAR-100 for these experiments. Finally, we also tested our methods' ability to learn when the unlabeled pool contained out-of-distribution samples, a case which, to the best of our knowledge, cannot be handled by any existing methods.

\noindent\textbf{Effect of Biased Initial Pool:} We first investigated the effect of bias that may be present in the initial labeled pool, $\mathcal{L}_0$. As stated in \cite{sinha2019variational}, bias can negatively impact the training of an active learner because it means that the initial labeled pool may not be representative of the true underlying data distribution.  Unless explicitly accounted for, this will cause a system to learn an incomplete, or biased, model of the latent space.  Following the protocol defined in \cite{sinha2019variational}, we removed all data points for $c$ classes from $\mathcal{L}_0$, thereby unbalancing the dataset and thus introducing bias. As shown in Fig.~\ref{fig:mixeddifferentBudgets}(a), our method outperformed VAAL, Core-set, and random sampling w.r.t selecting useful data points from classes that were underrepresented in the initial labeled pool. Models [$M_1^{sgd}, M_1^{adam}, M_2^{sgd}, M_2^{adam}$] achieved accuracies of [53.35\%, 60.54\%, 61.36\%, 61.55\%], respectively, when $c$ = 20 and [54.72\%, 60.79\%, 61.53\%, 61.57] when $c$ = 10 (as noted above, $c$ is the number of classes from which to exclude data).  VAAL, by comparison, came in second, followed by Core-set, exhibiting accuracies [46.91\%, 46.55\%] for $c$=20 and [47.10\%, 47.63\%] for $c$=20, respectively.  Random sampling achieved an accuracy of 45.33\% for $c$ = 10 and 45.87\% for $c$ = 20.

\noindent\textbf{Effect of Budget Size on Performance:} In this section, we tested the effect of different budget sizes $b$ on performance. Specifically,
we investigated the effect of budgets of size $b$ = 5\% and $b$ = 10\%, referring to percentage of samples taken from $\mathcal{D}_{train}$ at each stage of learning. As shown in Fig.~\ref{fig:mixeddifferentBudgets}(b), our model outperformed VAAL, Core-Set, Ensemble, and random sampling over both the budget sizes. VAAL comes in second followed by Core-set and  Ensemble.  Models [$M_1^{sgd},M_1^{adam},M_2^{sgd},M_2^{adam}$] achieve accuracies of [61.52\%, 61.57\%, 61.07\%, 61.82\%] for $b$ = 10 and [54.32\%, 60.68\%, 61.29\%, 61.9\%] for $b$ = 20.

% \begin{figure*}
%   \centering
%   \includegraphics[width=15cm,height=5.5cm]{images/noisypool-noisyunlabeled.png}
%   \caption{ Robustness of our approach on classification tasks to (a) Noisy
%   Oracle on CIFAR100 (left), (b) Mixed Unlabeled pool on CIFAR10 (right),. M1
%   indicates our model \eqref{eqn:M1Loss} and M2 indicates our model
%   \eqref{eqn:M2Loss}. All the Legend names are in descending order of final
%   accuracies (left). Best visible in color. Data and code required to reproduce
%   are provided in our supplementary code.}
%   \label{fig:mixednoisyoracle}
% \end{figure*}

\begin{figure}[h]
  \includegraphics[width=8cm,height=8cm]{images/noisy_oracle.png}
   \caption{ Robustness of our approach on CIFAR-100 given a noisy oracle. $M_1$
  indicates our model \eqref{eqn:M1Loss} and $M_2$ indicates our model
  \eqref{eqn:M2Loss}. All legend names are in descending order of final accuracies.}
  \label{fig:mixednoisyoracle}
%   \label{fig:differentBudgets}
\end{figure}
\noindent\textbf{Noisy Oracle:} Next, we investigated the performance of our approach in the presence of noisy data caused by an inaccurate, or noisy oracle. As in \cite{sinha2019variational}, we assumed that incorrect labels can be caused by the natural ambiguity which exists between examples drawn from 2 separate classes, rather than adversarial attacks. CIFAR-100 has both classes and super-classes, so, following \cite{sinha2019variational}, we randomly modified the labels of either 10\%, 20\% or 30\% of the samples by replacing them with a label from another class within the same super-class. As shown in Fig.~\ref{fig:mixednoisyoracle}, our models consistently outperformed existing approaches \textit{across all noise levels}. In other words, our $M_1$ model with 30\% noise was \textit{more accurate} than VAAL, etc. with 10\% noise.

\noindent\textbf{Sampling Time Analysis} We also replicated the sampling time analysis put forth in \cite{sinha2019variational}. Table \ref{tab:sampling_time} shows that our method is competitive with other state-of-the-art techniques w.r.t. execution time, thereby offering strong empirical evidence that our method offers large performance advantages with minimal additional computation.

\begin{table}[h]
\caption{Sampling Time Analysis: Mean time to select a sample from the unlabeled pool of CIFAR-100.} 
\begin{center}
\begin{tabular}{lc}
\textbf{Method}  &\textbf{Time (Seconds)} \\
\hline \\
VAAL         &10.69 \\
\textbf{Uncertainty sampling} &\textbf{10.89} \\
DBAL             &11.05 \\
\textbf{Weibull sampling}   &\textbf{20.41} \\
Ensembles w. VarR  &20.48\\
Core-set &75.33 \\
MC-Dropout &83.65  \\
\end{tabular}
\end{center}
% \caption{Sampling time}
\label{tab:sampling_time}
\end{table}

% (i dont think this is necessary) In the case of VAAL a separate VAE, Discriminator is used as part of their sampling strategy.

%  \cite{sinha2019variational}, Core-set \cite{sener2017active} ,
%   Ensembles w. VarR \cite{powerOfEnsemblesForActiveLearning}, MC-Dropout
%   \cite{gal2016dropout}, DBAL \cite{gal2017deep}, and Random Sampling. M1
%   indicates our model with Encoder and Classifier and M2 indicates our model
%   with encoder-decoder and classifier Best visible in color. Data and code
%   required to reproduce are provided in our code repository.
  
\begin{figure}[h]
  \centering
  \includegraphics[width=8cm]{images/n.png}
  \caption{Robustness of our approach on CIFAR10 classification tasks when the unlabeled pool includes samples from either the SVHN, KMNIST, or FashionMNIST datasets. The first three curves used the $M_2$ classifier, while the ones with the 'Random' subscript used random sampling. Our results confirm that our approach significantly outperforms this baseline.}
  \label{fig:iiid}
\end{figure}

% , CIFAR100 compared
%   to VAAL \cite{sinha2019variational}, Core-set \cite{sener2017active} ,
%   Ensembles w. VarR \cite{powerOfEnsemblesForActiveLearning}, MC-Dropout
%   \cite{gal2016dropout}, DBAL \cite{gal2017deep}, and Random Sampling. M1
%   indicates our model with Encoder and Classifier and M2 indicates our model
%   with encoder-decoder and classifier Best visible in color. Data and code
%   required to reproduce are provided in our code repository.

\textbf{Out-of-distribution samples in unlabeled pool:} Finally, we also tested an extreme case of active learning in which data samples from other datasets are mixed into the current unlabeled pool. We used CIFAR-10 for these experiments. Here, we intentionally added 20\% data (10,000 images) from other datasets to the unlabeled pool; thus, the network must distinguish not only between informative and non-informative samples but also distinguish \textit{in-distribution} data samples from \textit{out-of-distribution} samples. Whenever our model selected an OOD sample, the oracle discarded the sample, thus reducing the overall budget size. The discarded samples were placed back in the unlabeled pool (so the total number of OOD samples remained at 10,000). 

Figure~\ref{fig:iiid} shows our $M_2$ method's performance on CIFAR-10 when the unlabeled pool contained images from either SVHN, KMNIST, or FashionMNIST. Here, we used Weibull sampling (Sec.~\ref{sec:WiebullSampling}) due to its better outlier rejection compared to uncertainty sampling. For comparison, we also tested random sampling as a baseline. Impressively, despite the presence of 20\% OOD samples, our method significantly outperformed existing state-of-the-art methods trained on the regular unlabeled pool (Fig.~\ref{fig:CF10CF100}). And its performance, regardless of the second dataset, was only slightly below the standard $M_2$ method.

% As you can see at
% the end of graph in the fig. \ref{fig:iiid}, the increase in the accuracy was lower because the unlabeled pool had a higher impact on the sampling methodology. We
% used our sampling strategy 2 in this scenario as our sampling technique have ability of choosing values based on the range of the confidence level.we set our threshold to be in range of between 0.5 to 0.8 as this will help in eliminating
% the total outliers and pick the ones which are most useful for the model.

% \subsection{Choice of Network Architecture}

% \begin{table}[h]
%   \centering
%   \begin{tabular}{ |M{1.5cm}|M{1cm}|M{1.8cm}|M{1cm}|
%   M{1.8cm}|M{1.3cm}|M{1.2cm}|M{1.2cm}| }
%     \hline
%     \multicolumn{8}{|c|}{Sampling Time Analysis}
%     \\
%     \hline
%     \textbf{Method}                                            & VAAL
%     \cite{sinha2019variational}                           & Our Sampling Method
%     1                                      & DBAL  \cite{gal2017deep} & Our
%     Sampling Method 2                                      & Ensembles w. VarR
%     \cite{powerOfEnsemblesForActiveLearning} & Core-set \cite{sener2017active}
%     & MC-Dropout  \cite{gal2016dropout} \\
%     \hline
%     \textbf{Sampling Time}                                     & 10.69 & 10.89 &
%     11.05 & 20.41 & 20.48 & 75.33
%     & 83.65                                   \\
%     \hline
    
%   \end{tabular}
%   \vspace{0.9em}

% \end{table}

\section{Conclusions and Future work}
\label{sec:conclusions}
We have presented a novel approach for deep active learning using open-set recognition. To the best of our knowledge, we are the first to merge AL with OSR. Extensive experiments conducted over several image classification datasets have verified the effectiveness of our approach and established new state-of-the-art benchmarks. Specifically, we empirically demonstrated that the samples most worth labeling are those which are most different from the current labeled pool. Training on such samples allows the model to learn features underrepresented in the existing training data. We extensively tested the robustness of our approach using different budget sizes, a noisy oracle, and an unlabeled pool comprised of multiple datasets. In future work, we plan to test our approach on continual learning problems, in which the system must learn to solve different problems over time. We also plan to test our method on other problems, including image segmentation and document classification.

% focus on merging the distinct fields of Active Learning and Continual Learning in an effort to break ground on systems which learn actively, continually and expand the current setup to image segmentation methods.

% \subsubsection*{Acknowledgements}
% All acknowledgments go at the end of the paper, including thanks to reviewers who gave useful comments, to colleagues who contributed to the ideas, and to funding agencies and corporate sponsors that provided financial support. 
% To preserve the anonymity, please include acknowledgments \emph{only} in the camera-ready papers. 

% \subsubsection*{References}

\bibliography{reference}
\bibliographystyle{icml2021}

\end{document}
